# Supplementary material for: Multiple-bounce Smith Microfacet BRDFs using the Invariance Principle
Source: arXiv:2302.03408 source file (2023-09-02)
Supplement: Supplementary file 1 [file paper_appendix.tex]

%-------------------------------------%
\section{Formulation for medium slab}

\label{appendix:mediaSlab}
\subsection{Reflection}
% \textbf{:}
\begin{equation}
\begin{aligned}
&\rho _r\left(\omega_{i}, \omega_{o}\right) = \frac{1}{\Lambda\left(-\omega_{i}\right)+\Lambda\left(\omega_{o}\right)}\bigg(v\left(\omega_{i}, \omega_{o}\right)+\\
&\int_{\Omega^+}\Big(\rho _r\left(\omega_{i}, \omega\right) v\left(\omega, \omega_{o}\right)+v\left(\omega_{i},-\omega\right) \rho _r\left(-\omega, \omega_{o}\right)\Big) \mathrm{d} \omega \\
&+\int_{\Omega^+} \int_{\Omega^+}\Big(\rho _r\left(\omega_{i}, \omega_{1}\right) v\left(\omega_{1},-\omega_{2}\right)\rho _r\left(-\omega_{2}, \omega_{o}\right)-\\
&\rho _t\left(\omega_{i},-\omega_{1}\right) v\left(-\omega_{1}, \omega_{2}\right) \rho _t\left(-\omega_{2}, -\omega_{o}\right)\Big) \mathrm{d} \omega_{1} \mathrm{~d} \omega_{2}\bigg).
\end{aligned}
\end{equation}
% 透射：
\subsection{Transmission}
% \textbf{Transmission:}

\begin{equation}
\begin{aligned}
&\rho _t\left(\omega_{i}, \omega_{o}\right) = \delta\left(\left\|\omega_{i}-\omega_{o}\right\|\right) e^{-T \Lambda\left(-\omega_{i}\right)}+\frac{1}{\Lambda\left(-\omega_{i}\right)+\Lambda\left(\omega_{o}\right)}\\
&\bigg(\int_{\Omega^+}\Big(v\left(\omega_{i},-\omega\right) \rho_t\left(-\omega, \omega_{o}\right)-\rho_t\left(\omega_{i},-\omega\right) v\left(-\omega, \omega_{o}\right)\Big) \mathrm{d} \omega \\
&+\int_{\Omega^+} \int_{\Omega^+}\Big(\rho_r\left(\omega_{i}, \omega_{1}\right) v\left(\omega_{1},-\omega_{2}\right)\rho_t\left(-\omega_{2}, \omega_{o}\right)-\\
&\rho_t\left(\omega_{i},-\omega_{1}\right) v\left(-\omega_{1}, \omega_{2}\right) \rho_r\left(-\omega_{2}, -\omega_{o}\right)\Big) \mathrm{d} \omega_{1} \mathrm{~d} \omega_{2}\bigg).
\end{aligned}
\end{equation}

% \added{将 delta transmission 项带入积分，与一次散射组合，便可得到与 SpongeCake 一致的结果。}
